# Supplementary material for: Liquid crystal skyrmions as elastic multipoles
Source: arXiv:2410.03967 ancillary file (2024-10-04)
Supplement: Supplementary file 1 [file SM.pdf]

# Supplementary Information for Liquid crystal skyrmions as elastic multipoles

Allison W. Teixeira,[1,2,3] Cristóvão S. Dias,[1,2] and Mykola Tasinkevych[4,5]

[1] *Centro de Física Teórica e Computacional, Faculdade de Ciências, Universidade de Lisboa, 1749-016 Lisboa, Portugal*

[2] *Departamento de Física, Faculdade de Ciências, Universidade de Lisboa, 1749-016 Lisboa, Portugal*

[3] *Instituto de Alta Investigación, Universidad de Tarapacá, Casilla 7D, Arica, Chile*

[4] *SOFT Group, School of Science and Technology, Nottingham Trent University, Clifton Lane, Nottingham NG11 8NS, United Kingdom*

[5] *International Institute for Sustainability with Knotted Chiral Meta Matter, Hiroshima University, Higashihiroshima 739-8511, Japan.*

## CONTENTS

Supplementary Note 1. The Green's function for a circular particle 3

Supplementary Note 2. Effective elastic torque on a particle due to the far field director 5

Supplementary Note 3. The Green's function for two circular particles 6

References 10

### Supplementary Note 1. The Green's function for a circular particle

The Green's function $G(\mathbf{r}', \mathbf{r})$ for Laplace's equation with Dirichlet condition has a physical meaning of the Coulomb potential created by a unit positive point charge placed at $\mathbf{r}'$ when the boundary of the domain is maintained at zero electrostatic potential. This fact is used to construct the Green's function by using the method of images [1]. Consider a circular particle of radius $a$ which is centred at the origin of the $(x, y)$ plane as shown in Fig. S1. We denote the particle perimeter by $\zeta$. The single particle Green's function $G_1(\mathbf{r}', \mathbf{r})$ is defined for $r > a$, and satisfy $G_1(\mathbf{r}', \mathbf{r}) = 0$ for $\mathbf{r}' \in \zeta$. In this case only one image is sufficient to construct $G_1(\mathbf{r}', \mathbf{r})$. We place a imaginary unit negative point charge at the mirror image $\mathbf{i}_1(\mathbf{r}')$ of the real point $\mathbf{r}'$ reflected across the boundary $\zeta$. $\mathbf{i}_1(\mathbf{r}')$ lays inside the particle and is given by

$$\mathbf{i}_1(\mathbf{r}') = \frac{a^2}{|\mathbf{r}'|^2}\mathbf{r}'. \tag{S1}$$

Then, according to the method of images

$$G_1(\mathbf{r}', \mathbf{r}) = G_0(|\mathbf{r} - \mathbf{r}'|) - G_0(|\mathbf{r} - \mathbf{i}_1(\mathbf{r}')|), \tag{S2}$$

where $G_0(|\mathbf{r} - \mathbf{r}'|) = \ln|\mathbf{r} - \mathbf{r}'|/2\pi$ corresponds to the Coulomb potential due to a unit point charge in free-space located at $\mathbf{r}'$. The explicit form reads

$$G_1(\mathbf{r}', \mathbf{r}) = \frac{1}{4\pi}\log\left(\frac{|\mathbf{r} - \mathbf{r}'|^2}{|\mathbf{r} - \mathbf{i}_1(\mathbf{r}')|^2}\frac{a^2}{|\mathbf{r}'|^2}\right). \tag{S3}$$

The director perturbations $n_\mu$ now can be calculated by plugging Eq. (S3) into Eq. (4), which renders

$$\int_\zeta n_\mu(\mathbf{r}')\left(\boldsymbol{\sigma}\cdot\nabla_{\mathbf{r}'}\right)G_1(\mathbf{r}', \mathbf{r})d\mathbf{r}' = -a\int_\zeta n_\mu(a,\phi)\,\partial_{r'}G(a,\phi,\mathbf{r})\,|_{r'=a}\,d\phi, \tag{S4}$$

where we introduced polar coordinates $(x', y') = (r'\cos\phi, r'\sin\phi)$, $n_\mu(a,\phi)$ is the distribution of the director perturbation on $\zeta$. The Poisson kernel in Eq. (S4) can be expanded in

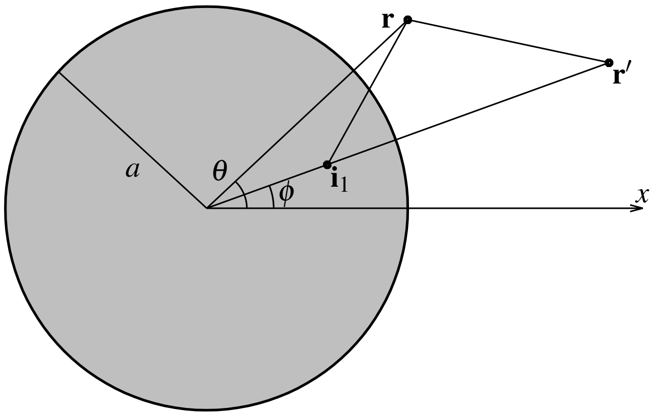


FIG. S1. **Representation of the LC soliton as a colloidal disc.** The inner region of the disc (grey colour) of radius $a$ contains all the strong distortions of the soliton. The region outside the disc perimeter $\zeta$ corresponds to the weak LC distortions, which can be described by the linearised model. $\mathbf{i}_1$ is the image of $\mathbf{r}'$ reflected across the disc perimeter $\zeta$ as if it were a mirror; $\theta$ and $\phi$ denotes the angles between $\mathbf{r}$ and $\mathbf{r}'$ and the $x$ axis, respectively.

powers of $(a/r) < 1$ as follows

$$n_\mu(r,\theta) = A_0^{(\mu)} + \sum_{n=1}^{\infty} \left(\frac{a}{r}\right)^n \left[A_n^{(\mu)} \cos(n\theta) + B_n^{(\mu)} \sin(n\theta)\right], \tag{S5}$$

where the coefficients are given by

$$A_0^{(\mu)} = \frac{1}{2\pi}\int_0^{2\pi} n_\mu(\theta)d\theta, \quad A_n^{(\mu)} = \frac{1}{\pi}\int_0^{2\pi} n_\mu(\theta)\cos(n\theta)d\theta,$$
$$B_n^{(\mu)} = \frac{1}{\pi}\int_0^{2\pi} n_\mu(\theta)\sin(n\theta)d\theta. \tag{S6}$$

By using the definitions in Eqs. (6) and (7), we find

$$\begin{aligned} q^{(\mu)} &= A_0^{(\mu)}, \\ p_x^{(\mu)} &= -\frac{a}{2}A_1^{(\mu)}, \quad p_y^{(\mu)} = -\frac{a}{2}B_1^{(\mu)}, \\ Q_{xy}^{(\mu)} &= \frac{a^2}{4}B_2^{(\mu)}, \quad Q_{xx}^{(\mu)} = -Q_{yy}^{(\mu)} = \frac{a^2}{4}A_2^{(\mu)}, \end{aligned} \tag{S7}$$

and the expansion of the director perturbations given by (S5) coincides with the main text multipole expansion (5).

## Supplementary Note 2. Effective elastic torque on a particle due to the far field director

Axisymmetric skyrmions realised at zero electric fields experience no torque because the far field director $\mathbf{n}_0 = \hat{\mathbf{z}}$. The elastic torques will emerge when $\mathbf{n}_0$ tilts away from $\hat{\mathbf{z}}$ as in the case of the bimerons. We denote by $\mathbf{p}_0^{(\mu)}$ and $\mathbf{Q}_0^{(\mu)}$ the elastic dipole and quadrupole moments which correspond to the free energy minimizing director configurations.

Here, we calculate the variation $\delta U_i$ of the free energy (8) of a single particle $i$ due to its rotation as a rigid body with respect to the fixed far field. This means that the LC texture and the director distribution on the particle perimeter $\zeta$ are "frozen" and rotated by small angle $\Delta\theta$ about the $z-$axis. The rotation results in variations of the dipole and quadrupole moments which we denote by $\Delta\mathbf{p}^{(\mu)}$ and $\Delta\mathbf{Q}^{(\mu)}$, respectively. The goal is to express $\delta U_i$ in terms of the equilibrium moments and their variations. To this end we write the functional differential of $U_i$ when $n_\mu$ varies along $\zeta$ as follows

$$\delta U_i = k \int_\zeta \int_\zeta \Delta n_\mu(\mathbf{r}') u_i(\mathbf{r}'\mathbf{r}) n_\mu(\mathbf{r}) d\mathbf{r}' d\mathbf{r}, \tag{S8}$$

where $\Delta n_\mu(\mathbf{r}') = n_\mu(r', \theta' - \Delta\theta') - n_\mu(\mathbf{r}')$ is the difference between the rotated and equilibrium perturbations. Equation (S8) can be rewritten by using main text equation (4) in the following form

$$\delta U_i = -k \int_\zeta n_\mu(\mathbf{r}) \left(\boldsymbol{\sigma}_\mathbf{r} \cdot \nabla_\mathbf{r}\right) \times \left[\int_\zeta \Delta n_\mu(\mathbf{r}') \left(\boldsymbol{\sigma}_{\mathbf{r}'} \cdot \nabla_{\mathbf{r}'}\right) G_1(\mathbf{r}', \mathbf{r}) d\mathbf{r}'\right] d\mathbf{r}. \tag{S9}$$

The Poisson kernel in the square brackets can be expanded in powers of $(a/r) < 1$, similarly

as in the previous note when passing from (S4) to (S5), leading to

$$\Delta n_\mu(r,\theta) = \sum_{n=1}^{\infty} \left(\frac{a}{r}\right)^n \left[\Delta A_n^{(\mu)} \cos(n\theta) + \Delta B_n^{(\mu)} \sin(n\theta)\right], \tag{S10}$$

where the $\Delta$-ed expansion coefficients are

$$\begin{aligned} \Delta A_n^{(\mu)} &= \frac{1}{\pi}\int_0^{2\pi} \Delta n_\mu(\theta)\cos(n\theta)d\theta, \\ \Delta B_n^{(\mu)} &= \frac{1}{\pi}\int_0^{2\pi} \Delta n_\mu(\theta)\sin(n\theta)d\theta. \end{aligned} \tag{S11}$$

Finally, the remaining derivative in Eq. (S9) can be calculated easily using Eq. (S4), which gives

$$\delta U_i = -4\pi k \sum_{n=1}^{\infty} n \left(\Delta A_n^{(\mu)} A_{0n}^{(\mu)} + \Delta B_n^{(\mu)} B_{0n}^{(\mu)}\right). \tag{S12}$$

$A_{0n}^{(\mu)}, B_{0n}^{(\mu)}$ above are the expansion coefficients of the equilibrium director perturbations. Main text equation (10) is obtained by using Eqs. (S7) in Eq. (S12).

**Supplementary Note 3. The Green's function for two circular particles**

The two particlex Green's function can not be calculated analytically, because to satisfy Dirichlet boundary condition on the both particle surface $\zeta_1$ and $\zeta_2$, see Fig. S2, an infinite number of images must be considered, i.e. in addition to the two images $\mathbf{i}_1(\mathbf{r}')$ and $\mathbf{i}_2(\mathbf{r}')$ of point $\mathbf{r}'$ reflected across the boundaries $\zeta_1$ and $\zeta_2$ we must also include secondary, ternary, etc. images of $\mathbf{r}'$. Here, we consider only two secondary images. The image of $\mathbf{i}_1(\mathbf{r}')$ reflected across the surface $\zeta_2$ is denoted as $\mathbf{i}_{12}(\mathbf{r}')$, and the image of $\mathbf{i}_2(\mathbf{r}')$ reflected across $\zeta_1$ is denoted as $\mathbf{i}_{21}(\mathbf{r}')$, see Fig. S2. Then, the two particles Green's function is approximated as follows

$$\begin{aligned} G_2(\mathbf{r}',\mathbf{r}) = G_0(|\mathbf{r}-\mathbf{r}'|) - G_0(|\mathbf{r}-\mathbf{i}_1(\mathbf{r}')|) - G_0(|\mathbf{r}-\mathbf{i}_2(\mathbf{r}')|) + \\ G_0(|\mathbf{r}-\mathbf{i}_{21}(\mathbf{r}')|) + G_0(|\mathbf{r}-\mathbf{i}_{12}(\mathbf{r}')|) + ... \end{aligned} \tag{S13}$$

Let $\mathbf{O}_1$ and $\mathbf{O}_2$ be the radius vectors of the centers of particle 1 and 2, respectively. We also introduce radius vectors $\mathbf{C}_1 \in \zeta_1$ and $\mathbf{C}_2 \in \zeta_2$ of points belonging to the boundaries of particle 1 and 2. In main text equation (11) the double integral runs over all pairs $(\mathbf{C}_1, \mathbf{C}_2)$. We note that $\mathbf{C}_1 = \mathbf{O}_1 - a_1\boldsymbol{\sigma}_1$ and $\mathbf{C}_2 = \mathbf{O}_2 - a_2\boldsymbol{\sigma}_2$, recall that the unit normal vectors $\boldsymbol{\sigma}_i$ point towards $\mathbf{O}_i$. The radius vectors of the first order images $\mathbf{i}_i(\mathbf{r}')$ of point $\mathbf{r}'$ can be obtained from the following expressions

$$\mathbf{i}_1(\mathbf{r}') - \mathbf{O}_1 = \gamma_1(\mathbf{r}' - \mathbf{O}_1), \quad \gamma_1 = \frac{a_1^2}{|\mathbf{r}' - \mathbf{O}_1|^2}, \tag{S14}$$

$$\mathbf{i}_2(\mathbf{r}') - \mathbf{O}_2 = \gamma_2(\mathbf{r}' - \mathbf{O}_2), \quad \gamma_2 = \frac{a_2^2}{|\mathbf{r}' - \mathbf{O}_2|^2}. \tag{S15}$$

The second order images satisfy

$$\mathbf{i}_{12}(\mathbf{r}') - \mathbf{O}_2 = \gamma_{12}(\mathbf{i}_1(\mathbf{r}') - \mathbf{O}_2), \quad \gamma_{12} = \frac{a_2^2}{|\mathbf{i}_1(\mathbf{r}') - \mathbf{O}_2|^2}, \tag{S16}$$

$$\mathbf{i}_{21}(\mathbf{r}') - \mathbf{O}_1 = \gamma_{21}(\mathbf{i}_2(\mathbf{r}') - \mathbf{O}_1), \quad \gamma_{21} = \frac{a_1^2}{|\mathbf{i}_2(\mathbf{r}') - \mathbf{O}_1|^2}. \tag{S17}$$

Now, we derive an approximate expression for the interaction kernel $u_{12}(\mathbf{r}', \mathbf{r})$ in (11) as an expansion in powers of $a_1/R$ and $a_2/R$, where $R = |\mathbf{R}|$. For convenience we provide below the expression for $u_{12}(\mathbf{r}', \mathbf{r})$ once more

$$u_{12}(\mathbf{r}', \mathbf{r}) = -\left[(\boldsymbol{\sigma}_2 \cdot \nabla_{\mathbf{r}'})(\boldsymbol{\sigma}_1 \cdot \nabla_{\mathbf{r}}) + (\boldsymbol{\sigma}_1 \cdot \nabla_{\mathbf{r}'})(\boldsymbol{\sigma}_2 \cdot \nabla_{\mathbf{r}})\right] G_2(\mathbf{r}', \mathbf{r}). \tag{S18}$$

Let us consider the first term in (S18). We start by calculating the derivative $(\boldsymbol{\sigma}_1 \cdot \nabla_{\mathbf{r}})$ and then taking the limit of the result as $\mathbf{r} \to \mathbf{C}_1$. Next we calculate the derivative $(\boldsymbol{\sigma}_2 \cdot \nabla_{\mathbf{r}'})$ followed by taking the limit $\mathbf{r}' \to \mathbf{C}_2$. Since point $\mathbf{r}'$ will be sent to $\zeta_2$, we may ignore in Eq. (S13) the term due to the second order image $\mathbf{i}_{12}(\mathbf{r}')$ because it is of a higher order, in $a_i/R$, as compared to the contributions of the first order images and the second image $\mathbf{i}_{21}(\mathbf{r}')$ [2]. With this approximation, the explicit expression for the Green's function reads

$$4\pi G_2(\mathbf{r}', \mathbf{r}) = \log\left(\gamma_1 \frac{|\mathbf{r} - \mathbf{r}'|^2}{|\mathbf{r} - \mathbf{i}_1(\mathbf{r}')|^2}\right) - \log\left(\gamma_{21} \frac{|\mathbf{r} - \mathbf{i}_2(\mathbf{r}')|^2}{|\mathbf{r} - \mathbf{i}_{21}(\mathbf{r}')|^2}\right). \tag{S19}$$

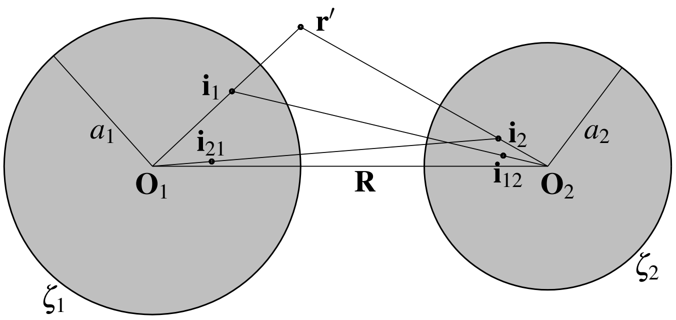


FIG. S2. **Two particles geometry and images of $\mathbf{r}'$.** Circular particle 1 of radius $a_1$ is centered at $\mathbf{O}_1$ and $\zeta_1$ denotes the particle perimeter, similar notations are used for particle 2. Vector $\mathbf{R} = \mathbf{O}_1 - \mathbf{O}_2$. The first order image of point $\mathbf{r}'$ reflected across $\zeta_1$ is located at $\mathbf{i}_1(\mathbf{r}')$, and the image reflected across $\zeta_2$ is located at $\mathbf{i}_2(\mathbf{r}')$. $\mathbf{i}_{12}(\mathbf{r}')$ and $\mathbf{i}_{21}(\mathbf{r}')$ are the second order images of $\mathbf{r}'$ such that $\mathbf{i}_{12}(\mathbf{r}')$ is the image of $\mathbf{i}_1(\mathbf{r}')$ reflected across $\zeta_2$ and $\mathbf{i}_{21}(\mathbf{r}')$ is the image of $\mathbf{i}_2(\mathbf{r}')$ reflected across $\zeta_1$.

After some algebra we find for the first term in (S18)

$$\lim_{\mathbf{r}'\to\mathbf{C}_2} (\boldsymbol{\sigma}_2 \cdot \nabla_{\mathbf{r}'}) \lim_{\mathbf{r}\to\mathbf{C}_1} (\boldsymbol{\sigma}_1 \cdot \nabla_{\mathbf{r}}) G_2(\mathbf{r}',\mathbf{r}) = -\frac{1}{2\pi a_1 a_2} \frac{a_1^2 - |\mathbf{R} - a_2\boldsymbol{\sigma}_2|^2}{|\mathbf{C}_2 - \mathbf{C}_1|^2}. \tag{S20}$$

The expression for the second term in Eq. (S18) follows from Eq. (S20) by changing $1 \to 2$ and $2 \to 1$ as well as replacing $\mathbf{R}$ with $-\mathbf{R}$. This renders

$$\lim_{\mathbf{r}'\to\mathbf{C}_1} (\boldsymbol{\sigma}_1 \cdot \nabla_{\mathbf{r}'}) \lim_{\mathbf{r}\to\mathbf{C}_2} (\boldsymbol{\sigma}_2 \cdot \nabla_{\mathbf{r}}) G_2(\mathbf{r}',\mathbf{r}) = -\frac{1}{2\pi a_1 a_2} \frac{a_2^2 - |\mathbf{R} + a_1\boldsymbol{\sigma}_1|^2}{|\mathbf{C}_2 - \mathbf{C}_1|^2}. \tag{S21}$$

To obtain the total interaction kernel $u_{12}$, we add (S20) and (S21) and use $\mathbf{C}_2 - \mathbf{C}_1 = \mathbf{R} + a_1\boldsymbol{\sigma}_1 - a_2\boldsymbol{\sigma}_2$ which gives

$$u_{12} = -\frac{1}{\pi a_1 a_2} \frac{\mathbf{R} \cdot (\mathbf{R} + a_1\boldsymbol{\sigma}_1 - a_2\boldsymbol{\sigma}_2)}{|\mathbf{R} + a_1\boldsymbol{\sigma}_1 - a_2\boldsymbol{\sigma}_2|^2}. \tag{S22}$$

This kernel is similar to the one found for colloids dispersed in three dimensional nematic LC [2], with the only difference that in the later case $u_{12} \propto |\mathbf{C}_2 - \mathbf{C}_1|^{-3}$. Next, we expand

the r.h.s. of (S22) in powers of $a_1/R$ and $a_2/R$, which provides

$$
\begin{aligned}
\pi a_1 a_2 \;\; u_{12} \;\; (\mathbf{C}_1, \mathbf{C}_2) = -1 - \frac{a_2 (\mathbf{u}\cdot\boldsymbol{\sigma}_2) - a_1 (\mathbf{u}\cdot\boldsymbol{\sigma}_1)}{R} \\
- \;\; \frac{2a_1 a_2 \left[(\boldsymbol{\sigma}_1\cdot\boldsymbol{\sigma}_2) - 2(\mathbf{u}\cdot\boldsymbol{\sigma}_1)(\mathbf{u}\cdot\boldsymbol{\sigma}_2)\right] + a_1^2\left[2(\mathbf{u}\cdot\boldsymbol{\sigma}_1)^2 - 1\right] + a_2^2\left[2(\mathbf{u}\cdot\boldsymbol{\sigma}_2)^2 - 1\right]}{R^2} \\
- \;\; \frac{3a_1 a_2 \left\{a_1\left[4(\mathbf{u}\cdot\boldsymbol{\sigma}_2)(\mathbf{u}\cdot\boldsymbol{\sigma}_1)^2 - 2(\mathbf{u}\cdot\boldsymbol{\sigma}_1)(\boldsymbol{\sigma}_1\cdot\boldsymbol{\sigma}_2) - (\mathbf{u}\cdot\boldsymbol{\sigma}_2)\right]\right\}}{R^3} \\
- \;\; \frac{3a_1 a_2 \left\{a_2\left[4(\mathbf{u}\cdot\boldsymbol{\sigma}_1)(\mathbf{u}\cdot\boldsymbol{\sigma}_2)^2 - 2(\mathbf{u}\cdot\boldsymbol{\sigma}_2)(\boldsymbol{\sigma}_1\cdot\boldsymbol{\sigma}_2) - (\mathbf{u}\cdot\boldsymbol{\sigma}_1)\right]\right\}}{R^3} \\
- \;\; \frac{2a_1^2 a_2^2 \left\{24(\mathbf{u}\cdot\boldsymbol{\sigma}_1)^2(\mathbf{u}\cdot\boldsymbol{\sigma}_2)^2 - 16(\mathbf{u}\cdot\boldsymbol{\sigma}_1)(\mathbf{u}\cdot\boldsymbol{\sigma}_2)(\boldsymbol{\sigma}_1\cdot\boldsymbol{\sigma}_2) - 4(\mathbf{u}\cdot\boldsymbol{\sigma}_1)^2\right\}}{R^4} \\
- \;\; \frac{2a_1^2 a_2^2 \left\{-4(\mathbf{u}\cdot\boldsymbol{\sigma}_2)^2 + 2(\boldsymbol{\sigma}_1\cdot\boldsymbol{\sigma}_2)^2 + 1\right\}}{R^4} - ..., 
\end{aligned}
\tag{S23}
$$

where $\mathbf{u} = \mathbf{R}/R$. Finally, we substitute the expansion in (S23) into (11), and by using the definitions of the elastic multipoles in Eqs. (6) and (7), we obtain for the interaction $U_{12}$ the expression in terms of multipole-multipole potentials as given by Eq. (13).

## REFERENCES

[1] N. Asmar, *Partial Differential Equations with Fourier Series and Boundary Value Problems* (Pearson Prentice Hall, 2005).

[2] V. M. Pergamenshchik and V. O. Uzunova, Elastic charge density representation of the interaction via the nematic director field, Eur. Phys. J. E **23**, 161 (2007).
